# Supplementary material for: Sub-Optimal Moving Horizon Estimation in Feedback Control of Linear Constrained Systems
Source: arXiv:2304.06216 source file (2023-04-13)
Supplement: Supplementary file 2 [file appendix_new.tex]

We define some longer terms here for clarity. Let
% \begin{subequations}
%  \begin{flalign}
%   &  M_1 = \frac{1}{2} \left(H^{-1}-H^{-1} T^{T}\left(T H^{-1} T^{T}\right)^{-1} T H^{-1}\right),  \label{M1 define}  \\
%  &  M_2 = H^{-1} T^{T}\left(T H^{-1} T T\right)^{-1}.  \label{M2 define} 
% \end{flalign}
% \end{subequations}
%
\begin{align} \label{H T}
   H = \begin{bmatrix}
Q & 0 & 0 & 0 \\
 0& R &0  & 0 \\
0 & 0 & \ddots  &  0\\
0 & 0 & 0 & P \\
\end{bmatrix}, 
T =  \begin{bmatrix}
I &0 & 0 & 0 \\
A & B & -I &0  \\
 & \ddots  & \ddots  &  \\
0 & A & B & -I \\
\end{bmatrix}. 
\end{align}

\subsection{Lemma 1 Proof}
\begin{proof}
Consider a constraint of the form
\begin{align}
 & \mathbb{C}_{i}(\delta_t):=\left\{\left[D_i z - d_i, g_i\right]^\top \mid \| D_i z - d_i \|_{2} \leq  (1-\delta_t) g_i\right\}. 
\end{align}
Given the upperbound we have 
\begin{align}
   &\| D_i z^K_{\delta_t,t} - d_i - D_i z^*_{\delta_t,t} - d_i \| \\
    \leq & \| D_i \| \| z^K_{\delta_t,t} - z^*_{\delta_t,t}\| \\
    \leq & \| D_i \| \delta_t \theta.
\end{align}
We want to show 
\begin{align}
    \|  D_i z^K_{\delta_t,t} - d_i \| \leq g_i.
\end{align}

Let
\begin{align}
    \lfloor h_x \rfloor & = \min h_x, \\
    \lfloor h_u \rfloor & = \min h_u, \\
    r_f & = { h_f}  {\overline{\lambda}(P)  }^{-\frac{1}{2}},
\end{align}
where $r_f$ denotes the smallest radii of the ellipsoid defined by $\mathcal{X}_f(\delta_t)$.

The constraint tightening rule that we design needs to guarantee
\begin{align} 
& \| x^{k}_{\delta_t,i}(\eta) - x^{*}_{\delta_t,i}(\eta) \|     \leq  \left\|{z}^{k}_{\delta_t}-{z}^{*}_{\delta_t}\right\| \leq \delta_t \lfloor h_x \rfloor, \\
& \| u^{k}_{\delta_t,i}(\eta) - u^{*}_{\delta_t,i}(\eta) \|     \leq  \left\|{z}^{k}_{\delta_t}-{z}^{*}_{\delta_t}\right\| \leq \delta_t \lfloor h_u \rfloor, \\
& \| x^k_{\delta_t} (N) - x^{*}_{\delta_t} (N)\|     \leq  \left\|{z}^{k}_{\delta_t}-{z}^{*}_{\delta_t} \right\| \leq \delta_t r_f. 
\end{align}
By satisfying the above, we can show the following:

\textbf{Ellipsoidal constraints:} 

Regarding the quadratic terminal constraint, we have
\begin{align}
    \| & x^k_{\delta_t}(N) \|_P \nonumber\\ 
    &  \leq \| x^k_{\delta_t}(N) - x^*_{\delta_t}(N) + x^*_{\delta_t}(N) \|_P \\
  &  \leq \| x^k_{\delta_t}(N) - x^*_{\delta_t}(N) \|_P + \| x^*_{\delta_t}(N) \|_P \\
    &  \leq  {\overline{\lambda}(P)  }^{\frac{1}{2}} \| x^k_{\delta_t}(N) - x^*_{\delta_t}(N) \| + (1-\delta_t) {h_f}  \\
&  \leq  {\overline{\lambda}(P)  }^{\frac{1}{2}} \delta_t r_f + (1-\delta_t) {h_f} \\
&  =  {\overline{\lambda}(P)  }^{\frac{1}{2}} \delta_t { h_f}  {\overline{\lambda}(P)  }^{-\frac{1}{2}} + (1-\delta_t) {h_f}  = {h_f}
\end{align}
which gives
\begin{equation}
     \| x^k_{\delta_t}(N) \|^2_P \leq h_f.
\end{equation}

Let 
\begin{equation}
    h = \min (\lfloor h_x \rfloor, \lfloor h_u \rfloor, r_f),
\end{equation}
our design goal is to satisfy
\begin{equation}
    \left\|{z}^{k}_{\delta_t}-{z}^{*}_{\delta_t} \right\| \leq \delta_t h.
\end{equation}
for $t \geq 0$, 
which we full-fill with a constraint-tightening update rule.

\end{proof}

\subsection{Proposition 1 Proof}
\begin{proof}
Since Assumption 2 holds, $\lambda_{\delta_t, t}$ is unique. 
Since

We show Lipschitz continuity properties of $\mathbb{P}(x_t,\delta_t)$ by formulating it as a parametric optimization problem
\begin{subequations} \label{simplified mpc}
\begin{align} 
 &\min_{z} \:  f(z,d_t(\delta_t)) = \| z \|^2_H \\
&E(z,d_t(\delta_t))  = 0 \\
&F(z,d_t(\delta_t)) \leq 0 
\end{align}
\end{subequations}
where $E(z,d)$ includes the initial and dynamic constraint and $F(z,d)$ includes the state, input, and terminal constraints.
The decision variable is $z = [\textbf{x},\textbf{u}]$
The time-varying parameter is $d_t(\delta_t) = [x_t,(1-\delta_t)h_{x},(1-\delta_t)h_{u},(1-\delta_t)^2 h_{f}]^{\top}$.
%
% We use $z^*_{\delta_t,t} = \operatorname{argmin}_{z} ( f(z,d_t(\delta_t)) )$ to denote the optimal solution to \eqref{simplified mpc}.

Since $f(z,d)$ is strongly convex, $F(z,d)$ is convex, $E(z,d)$ is affine, and all three are twice differentiable, the assumptions of [Wager 1969] are satisfied. Under further assumption that we only consider $x \in \Gamma_{{\infty}}$, we have 
\begin{equation}
  \|z_{\delta_1,1} - z_{\delta_2,2} \|  \leq L \| d_1 - d_2 \|.   
\end{equation}
The definition of $d$ leads to
\begin{align} \label{lemma 1 mid}
  \|&z_{\delta_1,1} - z_{\delta_2,2} \| \nonumber \\
   \leq & L \| x_1 - x_2 \| + L \|(1-\delta_1)h_x - (1-\delta_2)h_x \| \nonumber\\ 
   & + L \|(1-\delta_1)h_u - (1-\delta_2)h_u \| \nonumber\\
   & + L \|(1-\delta_1)^2 h_f - (1-\delta_2)^2 h_f\|.
\end{align}

When $\delta_1 = \delta_2$, we have the first claim.

When $x_1 = x_2$, we can plug 
\begin{align}
  &  L \|(1-\delta_1)h_x - (1-\delta_2)h_x \| \leq L \| h_x \| ( \| \delta_1\| + \| \delta_2 \| ), \\
 &L \|(1-\delta_1)h_u - (1-\delta_2)h_u \| \leq L \| h_u \| ( \| \delta_1\| + \| \delta_2 \| ),
\end{align}
and 
\begin{align}
  L \| & (1-\delta_1)^2 h_f -  (1-\delta_2)^2 h_f\| \\
 & \leq L h_f\|(1-\delta_1)^2 - (1-\delta_2)^2 \| \\
 & = L h_f \| \delta_1^2 - \delta_2^2 + 2 \delta_2 - 2 \delta_1\| \\
 & \leq 3 L h_f ( \| \delta_1\| +  \| \delta_2\| )
\end{align}
into \eqref{lemma 1 mid} to aquire the second claim. Notice the last inequality is true because $\delta^2 \leq \delta$ for $\delta \in [0,1)$.
\end{proof}

\subsection{Proposition 2 Proof}

\begin{proof}
It is obvious that 
\begin{equation} \label{t2_1}
    \|z_{t+1}\|_H  \leq  \|z^*_{t+1}\|_H + |  \|z_{t+1}\|_H - \|z^*_{t+1}\|_H |.
\end{equation}
We want to bound $ \|z^*_{t+1}\|_H $ and $|  \|z_{t+1}\|_H - \|z^*_{t+1}\|_H |$.

For $ \|z^*_{t+1}\|_H $:
Since \eqref{controlled system} is optimally-controlled the solution of $\mathbb{P}(x_t,0)$, we have
\begin{align} \label{l1_1}
          V(x^*_{t+1}) & \leq V(x_{t}) - \| x_{t} \|^2_Q.  
\end{align}
From \eqref{lips 1} and \eqref{uplowbound} we have
\begin{equation} \label{l1_2}
   \| x_{t+1} \|^2_Q \geq \underline{\lambda} (Q) \| x_{t+1}\|^2 \geq \frac{\underline{\lambda} (Q)}{L^2}  \| z_{t+1} \|^2,
\end{equation}
as well as 
\begin{equation} \label{l1_3}
    \| z_{t+1} \|^2 \geq \frac{1}{\overline{\lambda} (H) } \| z_{t+1} \|^2_H.
\end{equation}
Plugging \eqref{l1_2} and \eqref{l1_3} into \eqref{l1_1} sequentially gives
\begin{align} \label{l1_4}
    V(x^*_{t+1}) - V(x_{t})  & \leq - \frac{ \underline{\lambda} (Q) }{ L^2 \overline{\lambda} (H) } V(x_{t}).
\end{align}
Alternatively, we have
\begin{equation} \label{l1_5}
    V(x^*_{t+1}) \leq ( 1 - \frac{ \underline{\lambda} (Q) }{ L^2 \overline{\lambda} (H)}) V(x_{t}),
\end{equation}

For $|  \|z_{t+1}\|_H - \|z^*_{t+1}\|_H |$:
Using the reverse triangle inequality, we have 
\begin{equation} \label{l2_1}
     | \| z^*_{t+1} \|_H - \| z_{t+1} \|_H |^2 \leq \| z^*_{t+1} - z_{t+1}   \|^2_H.
\end{equation}
Applying \eqref{lips 1} and \eqref{uplowbound} to the r.h.s yields
\begin{align} 
     | \| z^*_{t+1} \|_H - \| z_{t+1} \|_H |^2  \leq \overline{\lambda}(H) \| z^*_{t+1} - z_{t+1}   \|^2 & 
     \\  \leq   \overline{\lambda}(H) L^2 \| x^*_{t+1} - x_{t+1}   \|^2, &
\end{align}
implying
\begin{equation} \label{l2_2}  
     | \| z^*_{t+1} \|_H - \| z_{t+1} \|_H | \leq  \sqrt{\overline{\lambda}(H)} L \| x^*_{t+1} - x_{t+1}  \|.
\end{equation}
Plugging \eqref{l2_3} into the above gives 
\begin{equation} \label{l2_4}
    \| \sqrt{V(x^*_{t+1})} - \sqrt{V(x_{t+1})} \| \leq  \sqrt{\overline{\lambda}(H)} L \| B \| \epsilon_{t}.
\end{equation}

Using \eqref{l1_5} and \eqref{l2_4} with \eqref{t2_1} gives the claim.
\end{proof}

\subsection{Proposition 3 Proof}
\begin{proof}
From the update rule \eqref{update rule of delta} and \eqref{delta x simplify} we immediately have the claim.
\end{proof}

\subsection{Proposition 4 Proof}
\begin{proof}
We start with 
\begin{align}
 & \epsilon_{t+1} =  \left\|z_{\delta_{t+1},{t+1}}^{k}-z_{{t+1}}^{*}  \right\| \\
= & \left\|z_{\delta_{t+1},{t+1}}^{k} - z_{\delta_{t+1},{t+1}}^{*}  + z_{\delta_{t+1},{t+1}}^{*} -z_{{t+1}}^{*}  \right\| \\
\leq & \|z_{\delta_{t+1},{t+1}}^{k} - z_{\delta_{t+1},{t+1}}^{*} \|  + \| z_{\delta_{t+1},{t+1}}^{*} -z_{{t+1}}^{*}  \| \\ 
\leq & {k^{-1} J } \|\lambda^{0}_{\delta_{t+1},{t+1}}-\lambda^{\star}_{\delta_{t+1},{t+1}}\| + \| z_{\delta_{t+1},{t+1}}^{*} -z_{{t+1}}^{*}  \|
\end{align}
and we want to upper-bound ${k^{-1} J } \|\lambda^{0}_{\delta_{t+1},{t+1}}-\lambda^{\star}_{\delta_{t+1},{t+1}}\|$ and $\| z_{\delta_{t+1},{t+1}}^{*} -z_{{t+1}}^{*}  \|$. For $\|\lambda^{0}_{\delta_{t+1},{t+1}}-\lambda^{\star}_{\delta_{t+1},{t+1}}\|$, we have 
\begin{align}
   \|\lambda^{0}_{\delta_{t+1},{t+1}}-\lambda^{\star}_{\delta_{t+1},{t+1}}\|  = \|\lambda^{k}_{\delta_{t},t}-\lambda^{\star}_{\delta_{t+1},{t+1}}\| 
\end{align}

\textcolor{red}{It is shown in \eqref{lemma 2 mid 5} that
\begin{align} 
 \left\|\lambda^{0}_{\delta_{t+1},{t+1}}-\lambda^{\star}_{\delta_{t+1},{t+1}}\right\| \leq & L  (  h  +  K )  \delta_{t} +   L K   \delta_{{t+1}}    \nonumber \\
 & +  L  \| \Delta x_{t} \|.
\end{align}}
Using the above to bound $\|\lambda^{0}_{\delta_{t+1},{t+1}}-\lambda^{\star}_{\delta_{t+1},{t+1}}\|$ and \eqref{lips 2} to bound $\| z_{\delta_{t+1},{t+1}}^{*} -z_{{t+1}}^{*}  \|$ we have 
\begin{align}
 \epsilon_{t+1} \leq &  {k^{-1} J } L  (  h  +  K )  \delta_{t} + ({k^{-1} J }   L K + LK )   \delta_{{t+1}} \nonumber \\
 & + {k^{-1} J } L  \| \Delta x_{t} \| 
\end{align}
Using \eqref{delta x simplify} to bound $\| \Delta x_{t} \|$ and \eqref{ISS function 3} to bound $\delta_{t+1}$ gives the claim after simplification.
\end{proof}

\subsection{Lemma 2 Proof}
\begin{proof} 
Given the ISS-Lyapunov functions for the subsystems
\begin{align}
    \psi(x_{t+1}) \leq & (1-\sigma_1) \psi(x_t) + \gamma_{1,2} \epsilon_{t}, \\
      \delta_{t+1} \leq  &  \gamma_{2,1} \psi(x_t) + \gamma_{2,3} \epsilon_{t}  + (1-\sigma_2) \delta_{t},\\
    \epsilon_{t+1} \leq & \gamma_{3,1} \psi(x_t)  + (1-\sigma_3) \epsilon_{t}  + \gamma_{3,2} \delta_{t},
\end{align}
positive invariance of $\Sigma$ can be guaranteed if 

(i)
\begin{align}
    \psi(x_{t+1}) \leq & (1-\sigma_1) \psi_{\bar{\delta}} +  \gamma_{1,2} \epsilon_{\bar{\delta}} \\
    \leq & \psi_{\bar{\delta}},
\end{align}
where the last inequality holds because we define 
\begin{align}
    \epsilon_{\bar{\delta}} = \frac{\sigma_1}{\gamma_{1,2}} \psi_{\bar{\delta}},
\end{align}

(ii) 
\begin{align}
    \delta_{t+1} \leq  & \gamma_{2,1} \psi_{\bar{\delta}} + \gamma_{2,3} \epsilon_{\bar{\delta}}  + (1-\sigma_2) \bar{\delta} \\
    \leq & \gamma_{2,1} \psi_{\bar{\delta}} + \gamma_{2,3} \frac{\sigma_1}{\gamma_{1,2}} \psi_{\bar{\delta}}  + (1-\sigma_2) \bar{\delta} \\
    \leq & \bar{\delta}
\end{align}
where the last inequality holds because we design A

(iii)
\begin{align}
     \epsilon_{t+1} \leq & \gamma_{3,1}  \psi_{\bar{\delta}}  + (1-\sigma_3)  \epsilon_{\bar{\delta}}  + \gamma_{3,2} \bar{\delta}\\
     \leq & \gamma_{3,1} \psi_{\bar{\delta}} + (1-\sigma_3)  \frac{\sigma_1}{\gamma_{1,2}} \psi_{\bar{\delta}}  + \gamma_{3,2} \bar{\delta} \\
     \leq & \epsilon_{\bar{\delta}}   \leq  \frac{\sigma_1}{\gamma_{1,2}} \psi_{\bar{\delta}}
\end{align}
where the last inequality holds because we design B

To design A and B is to have 
\begin{align}
    \gamma_{2,1} \psi_{\bar{\delta}} + \gamma_{2,3} \frac{\sigma_1}{\gamma_{1,2}} \psi_{\bar{\delta}}  + (1-\sigma_2) \bar{\delta} \leq  \bar{\delta} \\
    \gamma_{3,1} \psi_{\bar{\delta}} + (1-\sigma_3)  \frac{\sigma_1}{\gamma_{1,2}} \psi_{\bar{\delta}}  + \gamma_{3,2} \bar{\delta} \leq  \frac{\sigma_1}{\gamma_{1,2}} \psi_{\bar{\delta}}
\end{align}
which is to have 
\begin{align}
 & \frac{ \left( \gamma_{2,1}  + \gamma_{2,3} \frac{\sigma_1}{\gamma_{1,2}} \right) }{\sigma_2 } \psi_{\bar{\delta}} \leq \bar{\delta} \\
  &  \bar{\delta} \leq  \frac{\left( \sigma_3   \frac{\sigma_1}{\gamma_{1,2}}   - \gamma_{3,1} \right) }{ \gamma_{3,2}} \psi_{\bar{\delta}} 
\end{align}
which can be expressed as 
\begin{align}
 \frac{\gamma_{2,3} \sigma_1 + \gamma_{2,1} \gamma_{1,2}}{\gamma_{1,2}\sigma_2}   \psi_{\bar{\delta}} \leq  \bar{\delta} \leq     - \frac{  \gamma_{3,1}\gamma_{1,2} - \sigma_1 \sigma_3 }{ \gamma_{3,2}\gamma_{1,2} }  \psi_{\bar{\delta}} 
\end{align}
or 
\begin{align} \label{lm6 1}
    \ &   \frac{ \gamma_{1,2} \gamma_{2,3}  }{ \sigma_1 \sigma_2 -\gamma_{2,1}}   \bar{\delta}  \leq    \psi_{\bar{\delta}}   \leq  \frac{\gamma_{1,2} \sigma_3 }{ \gamma_{1,2}\gamma_{3,1} + \sigma_1 \gamma_{3,2}}   \bar{\delta}.
\end{align}

\end{proof}

\subsection{Proposition 5 Proof}
\begin{proof}
The main idea of the proof is to first show that
\begin{equation} \label{tight feasibility upper-bound}
 {k^{-1} J }  \left\|\lambda^{0}_{\delta_t,t}-\lambda^{*}_{\delta_t,t}\right\| \leq \delta_t h,
\end{equation}
where $h = \operatorname{min}(\lfloor h_x \rfloor, \lfloor h_u \rfloor ,r_f)$, is satisfied for $t \geq 0$ and so that
\begin{equation} \label{tight feasibility}
    \left\|{z}^{k}_{\delta_t,t}-{z}^{*}_{\delta_t,t}\right\| \leq \delta_t h
\end{equation}
is consequently satisfied, due to \eqref{upper bound sqrt}.
The second step is to show that satisfaction of \eqref{tight feasibility} results in satisfaction of $\mathbb{P}(x_t,0)$.

We prove \eqref{tight feasibility upper-bound} holds by considering the cases where $t = 0$ and $t = 1$, from which the proof for $t \geq 1$ naturally follows.

For $t = 0$, we already have
\begin{equation} 
    {{k^{-1} J } h^{-1}} \left\|\lambda^{\text{start}}_{\delta_0,0}-\lambda^{*}_{\delta_0,0} \right\| \leq \delta_0
\end{equation}
 from Algorithm 2.

For $t = 1$, we want to show
\begin{equation} \label{t=1 condition}
{{k^{-1} J } h^{-1}} 
    \left\|\lambda^{0}_{\delta_1,1}-\lambda^{*}_{\delta_1,1}\right\|
    \leq \delta_1 
\end{equation}

With warm-start $\lambda^{0}_{\delta_1,1} \leftarrow \lambda^{k}_{\delta_{0},0}$, we have that 
\begin{align}
 &  \|\lambda^{0}_{\delta_1,1}-\lambda^{*}_{\delta_1,1}\| 
 = \|\lambda^{k}_{\delta_{0},0}-\lambda^{*}_{\delta_1,1}\|  \\
  & = \|\lambda^{k}_{\delta_{0},0}
  -\lambda^{*}_{\delta_{0},0} +\lambda^{*}_{\delta_{0},0} 
 - \lambda^{*}_{0,0} +\lambda^{*}_{0,0}   - \lambda^{*}_{0,1} +\lambda^{*}_{0,1} \nonumber \\
&
  -\lambda^{*}_{\delta_1,1}\|  \\ 
& \leq \|\lambda^{k}_{\delta_{0},0}
  -\lambda^{*}_{\delta_{0},0} \|  + \| \lambda^{*}_{\delta_{0},0} 
 - \lambda^{*}_{0,0} \|   + \| \lambda^{*}_{0,0} 
 - \lambda^{*}_{0,1} \| \nonumber \\
 & + \| \lambda^{*}_{0,1}
  -\lambda^{*}_{\delta_1,1}\|  \\
  & \leq \|\lambda^{k}_{\delta_{0},0}
  -\lambda^{*}_{\delta_{0},0} \|  +  L K \| \delta_0\|  + L \| x_1 - x_0 \|+ L K \| \delta_1\|
\end{align}

\newpage

\textcolor{red}{We need a bound on $\| \|\lambda^{k}_{\delta_{0},0} -\lambda^{*}_{\delta_{0},0} \| \|$.}

For strongly convex functions we have 
\begin{align}
    f(y) \geq f(x) + \nabla f(x)^\top (y - x) + \frac{\mu}{2} \| y - x \|^2
\end{align}

For strongly concave functions we have 
\begin{align}
    f(y) \leq f(x) + \nabla f(x)^\top (y - x) - \frac{\mu}{2} \| y - x \|^2
\end{align}

The dual function we concern is
\begin{align*}
\mathbf{D}(\lambda)=&-  \lambda^{T}G \lambda+ g \lambda  -\frac{1}{4} h^{T} H^{-1} h-\sum_{i=1}^{M} I_{\lambda_{i} \in \mathbb{C}_{i}},
\end{align*}
where 
\begin{align*}
   G =  \frac{1}{4} C H^{-1} C^{T}  \;\textup{and}\; g = \frac{1}{2} h^{T} H^{-1} C^{T}+c^{T}.
\end{align*}

We want to show 
\begin{align*}
    \| \lambda^* - \lambda^K \|^2 & \leq \mathbf{D}(\lambda^*) - \mathbf{D}(\lambda^K) \\
   & = -\lambda^* G \lambda^* + \lambda^K G \lambda^K + g (\lambda^* - \lambda^K) 
\end{align*}

Let 
\begin{align}
    D(\lambda) = -\lambda G \lambda + g \lambda,
\end{align}
which is strongly concave.
We have 
\begin{align}
    D(\lambda^K) \leq D(\lambda^*) + \nabla D(\lambda^*)^\top (\lambda^K - \lambda^*) - \frac{\mu}{2} \| \lambda^K - \lambda^* \|^2
\end{align}
or 
\begin{align}
    D(\lambda^K) - D(\lambda^*) \leq  \nabla D(\lambda^*)^\top (\lambda^K - \lambda^*) - \frac{\mu}{2} \| \lambda^K - \lambda^* \|^2
\end{align}
or 
\begin{align}
    D(\lambda^*) - D(\lambda^K) \geq  -\nabla D(\lambda^*)^\top (\lambda^K - \lambda^*) + \frac{\mu}{2} \| \lambda^K - \lambda^* \|^2
\end{align}

Since moving away from $\lambda^*$ will only result in decrease in the function value, we have 
\begin{align}
    \nabla D(\lambda^*)^\top (\lambda^K - \lambda^*) < 0,
\end{align}
which means 
\begin{align}
    D(\lambda^*) - D(\lambda^K) &\geq  -\nabla D(\lambda^*)^\top (\lambda^K - \lambda^*) + \frac{\mu}{2} \| \lambda^K - \lambda^* \|^2 \\
    &\geq \frac{\mu}{2} \| \lambda^K - \lambda^* \|^2
\end{align}
Here
\begin{align}
    \mu = \overline{\lambda}(G)
\end{align}

\end{proof}

\subsection{Theorem 1 Proof}
